# Supplementary material for: Inverse Design of Multicomponent Assemblies
Source: arXiv:1801.02750 ancillary file (2018-02-19)
Supplement: Supplementary file 1 [file supplementary_material.pdf]

# Supplementary Material

## I. DERIVATION OF RELATIVE ENTROPY UPDATE SCHEME FOR A MULTICOMPONENT SYSTEM

In this section we provide a brief derivation of the update scheme shown in equation 1 in the main text. Without loss of generality, consider $i$ independent configurations of a two component system given by coordinates $\mathbf{R_i^{(A)}}$ and $\mathbf{R_i^{(B)}}$. Then in a canonical ensemble the probability of such configuration is given by the product of the Boltzmann factors

$$P(\mathbf{R_i^{(A)}}, \mathbf{R_i^{(B)}}|\boldsymbol{\theta}) = \prod_{i=1}^{M} \exp\left[-\beta U(\mathbf{R_i^{(A)}}, \mathbf{R_i^{(B)}}|\boldsymbol{\theta})\right]/Z(\boldsymbol{\theta}) \tag{S1}$$

where $U(\mathbf{R_i^{(A)}}, \mathbf{R_i^{(B)}})$ is the configuration energy, $\beta = 1/k_b T$, $T$ is temperature, $k_b$ is the Boltzmann constant, and $\boldsymbol{\theta}$ is a vector of the tunable potential parameters. As explained in detail in previous work[S1], given some desired configuration $(\mathbf{R^{(A)}}, \mathbf{R^{(B)}})$, we seek to maximize the likelihood of achieving this target given some parameters $\boldsymbol{\theta}$, i.e. we must maximize $P(\mathbf{R_i^{(A)}}, \mathbf{R_i^{(B)}}|\boldsymbol{\theta})$ with respect to $\boldsymbol{\theta}$. In practice, it is easier to maximize the log of the probability. Applying a log to eq. S1 and expanding we get

$$\frac{1}{M} \ln P(\mathbf{R_i^{(A)}}, \mathbf{R_i^{(B)}}|\boldsymbol{\theta}) = -\frac{1}{M} \sum_{i=1}^{M} \beta U(\mathbf{R_i^{(A)}}, \mathbf{R_i^{(B)}}|\boldsymbol{\theta}) - \ln Z(\boldsymbol{\theta}) \tag{S2}$$

We can now partition the system energy as a sum of independent self and cross component interactions as

$$U(\mathbf{R_i^{(A)}}, \mathbf{R_i^{(B)}}|\boldsymbol{\theta}) = U^{(A,A)}(\mathbf{R_i^{(A)}}|\boldsymbol{\theta}^{(A,A)}) + U^{(B,B)}(\mathbf{R_i^{(B)}}|\boldsymbol{\theta}^{(B,B)}) + U^{(A,B)}(\mathbf{R_i^{(A)}}, \mathbf{R_i^{(B)}}|\boldsymbol{\theta}^{(A,B)}) \tag{S3}$$

where $\boldsymbol{\theta}$ has been similarly split into self and cross parameters $\boldsymbol{\theta} = [\boldsymbol{\theta}^{(A,A)}, \boldsymbol{\theta}^{(B,B)}, \boldsymbol{\theta}^{(A,B)}]$ and plugging back into eq. S2 we get:

$$\begin{aligned} \frac{1}{M} \ln P(\mathbf{R_i^{(A)}}, \mathbf{R_i^{(B)}}|\boldsymbol{\theta}) = & \\ & -\frac{1}{M} \sum_{i=1}^{M} \beta U^{(A,A)}(\mathbf{R_i^{(A)}}|\boldsymbol{\theta}^{(A,A)}) \\ & -\frac{1}{M} \sum_{i=1}^{M} \beta U^{(B,B)}(\mathbf{R_i^{(B)}}|\boldsymbol{\theta}^{(B,B)}) \\ & -\frac{1}{M} \sum_{i=1}^{M} \beta U^{(A,B)}(\mathbf{R_i^{(A)}}, \mathbf{R_i^{(B)}}|\boldsymbol{\theta}^{(A,B)}) - \ln Z(\boldsymbol{\theta}) \end{aligned} \tag{S4}$$

which can be written

$$\langle \ln P(\mathbf{R^{(A)}}, \mathbf{R^{(B)}}|\boldsymbol{\theta})\rangle_{P_{\rm tgt}(\mathbf{R^{(A)}},\mathbf{R^{(B)}})} = \\ - \langle \beta U^{(A,A)}(\mathbf{R^{(A)}}|\boldsymbol{\theta}^{(A,A)})\rangle_{P_{\rm tgt}(\mathbf{R^{(A)}},\mathbf{R^{(B)}})} \\ - \langle \beta U^{(B,B)}(\mathbf{R^{(B)}}|\boldsymbol{\theta}^{(B,B)})\rangle_{P_{\rm tgt}(\mathbf{R^{(A)}},\mathbf{R^{(B)}})} \\ - \langle \beta U^{(A,B)}(\mathbf{R^{(A)}}, \mathbf{R^{(B)}}|\boldsymbol{\theta}^{(A,B)})\rangle_{P_{\rm tgt}(\mathbf{R^{(A)}},\mathbf{R^{(B)}})} - \ln Z(\boldsymbol{\theta}) \tag{S5}$$

where $\langle ... \rangle$ denotes ensemble average. In order to achieve a desired target probability we can optimize component parameters $\boldsymbol{\theta}^{k,k'}$, where $k,\ k' = A$ or $B$, using a gradient ascent approach of the form:

$$\boldsymbol{\theta}_{i+1} = \boldsymbol{\theta}_i + \alpha[\boldsymbol{\nabla}_{\boldsymbol{\theta}}\langle \ln P(\mathbf{R^{(A)}}, \mathbf{R^{(B)}}|\boldsymbol{\theta})\rangle]_{\boldsymbol{\theta}_i} \tag{S6}$$

where $\alpha$ is some scalar constant. Using $Z(\boldsymbol{\theta}) \equiv \int \exp[-\beta U(\mathbf{R^{(A)}}, \mathbf{R^{(B)}}|\boldsymbol{\theta})] d\mathbf{R^{(A)}} d\mathbf{R^{(B)}}$, where $d\mathbf{R^{(A)}} d\mathbf{R^{(B)}}$ indicate hyper-volume elements, and computing the gradient we have

$$\boldsymbol{\nabla}_{\boldsymbol{\theta}^{(A,A)}}\langle \ln P(\mathbf{R^{(A)}}, \mathbf{R^{(B)}}|\boldsymbol{\theta})\rangle_{P_{\rm tgt}(\mathbf{R^{(A)}},\mathbf{R^{(B)}})} = \\ - \langle \boldsymbol{\nabla}_{\boldsymbol{\theta}^{(A,A)}} \beta U^{(A,A)}(\mathbf{R^{(A)}}|\boldsymbol{\theta}^{(A,A)})\rangle_{P_{\rm tgt}(\mathbf{R^{(A)}},\mathbf{R^{(B)}})} + \langle \boldsymbol{\nabla}_{\boldsymbol{\theta}^{(A,A)}} \beta U^{(A,A)}(\mathbf{R^{(A)}}|\boldsymbol{\theta}^{(A,A)})\rangle_{P(\mathbf{R^{(A)}},\mathbf{R^{(B)}})} \tag{S7a}$$

$$\boldsymbol{\nabla}_{\boldsymbol{\theta}^{(B,B)}}\langle \ln P(\mathbf{R^{(A)}}, \mathbf{R^{(B)}}|\boldsymbol{\theta})\rangle_{P_{\rm tgt}(\mathbf{R^{(A)}},\mathbf{R^{(B)}})} = \\ - \langle \boldsymbol{\nabla}_{\boldsymbol{\theta}^{(B,B)}} \beta U^{(B,B)}(\mathbf{R^{(B)}}|\boldsymbol{\theta}^{(B,B)})\rangle_{P_{\rm tgt}(\mathbf{R^{(A)}},\mathbf{R^{(B)}})} + \langle \boldsymbol{\nabla}_{\boldsymbol{\theta}^{(B,B)}} \beta U^{(B,B)}(\mathbf{R^{(B)}}|\boldsymbol{\theta}^{(B,B)})\rangle_{P(\mathbf{R^{(A)}},\mathbf{R^{(B)}})} \tag{S7b}$$

$$\boldsymbol{\nabla}_{\boldsymbol{\theta}^{(A,B)}}\langle \ln P(\mathbf{R^{(A)}}, \mathbf{R^{(B)}}|\boldsymbol{\theta})\rangle_{P_{\rm tgt}(\mathbf{R^{(A)}},\mathbf{R^{(B)}})} = \\ - \langle \boldsymbol{\nabla}_{\boldsymbol{\theta}^{(A,B)}} \beta U(\mathbf{R^{(A)}}, \mathbf{R^{(B)}}|\boldsymbol{\theta}^{(A,B)})\rangle_{P_{\rm tgt}(\mathbf{R^{(A)}},\mathbf{R^{(B)}})} + \langle \boldsymbol{\nabla}_{\boldsymbol{\theta}^{(A,B)}} \beta U^{(A,B)}(\mathbf{R^{(A)}}, \mathbf{R^{(B)}}|\boldsymbol{\theta}^{(A,B)})\rangle_{P(\mathbf{R^{(A)}},\mathbf{R^{(B)}})} \tag{S7c}$$

which correspond to three independent equations for each parameter $k, k'$. Supposing isotropic pair interactions of the form $U^{(k,k)}(\mathbf{R^k}|\boldsymbol{\theta}^{(k,k)}) \equiv \frac{1}{2}\sum_{i\neq j}^{N^{(k)}} u^{(k,k)}(r_{i,j}^{(k)}|\boldsymbol{\theta}^{(k,k)})$ for self and $U^{(k,k')}(\mathbf{R^{k,k}}|\boldsymbol{\theta}^{(k,k')}) \equiv \sum_{i,j}^{N^{(k)},N^{(k')}} u^{(k,k')}(r_{i,j}^{(k,k')}|\boldsymbol{\theta}^{(k,k')})$ for cross interactions, we can then reduce the expressions in equation S7 to pair-density integral expressions given by

$$\boldsymbol{\nabla}_{\boldsymbol{\theta}^{(A,A)}}\langle \ln P(\mathbf{R^{(A)}}, \mathbf{R^{(B)}}|\boldsymbol{\theta})\rangle_{P_{\rm tgt}(\mathbf{R^{(A)}},\mathbf{R^{(B)}})} = \\ \pi\rho^{(A)}N^{(A)} \int drr[g^{(A,A)}(r|\boldsymbol{\theta}^{(A,A)}) - g_{\rm tgt}^{(A,A)}(r)]\boldsymbol{\nabla}_{\boldsymbol{\theta}^{(A,A)}}\beta u^{(A,A)}(r|\boldsymbol{\theta}^{(A,A)}) \tag{S8a}$$

$$\nabla_{\boldsymbol{\theta}^{(B,B)}} \langle \ln P(\mathbf{R}^{(\mathbf{A})}, \mathbf{R}^{(\mathbf{B})}|\boldsymbol{\theta}) \rangle_{P_{\mathrm{tgt}}(\mathbf{R}^{(\mathbf{A})}, \mathbf{R}^{(\mathbf{B})})} = \pi\rho^{(B)} N^{(B)} \int dr r [g^{(B,B)}(r|\boldsymbol{\theta}^{(B,B)}) - g_{\mathrm{tgt}}^{(B,B)}(r)] \nabla_{\boldsymbol{\theta}^{(B,B)}} \beta u^{(B,B)}(r|\boldsymbol{\theta}^{(B,B)}) \tag{S8b}$$

$$\nabla_{\boldsymbol{\theta}^{(A,B)}} \langle \ln P(\mathbf{R}^{(\mathbf{A})}, \mathbf{R}^{(\mathbf{B})}|\boldsymbol{\theta}) \rangle_{P_{\mathrm{tgt}}(\mathbf{R}^{(\mathbf{A})}, \mathbf{R}^{(\mathbf{B})})} = 2\pi\rho^{(A)}\rho^{(B)} V \int dr r [g^{(A,B)}(r|\boldsymbol{\theta}^{(A,B)}) - g_{\mathrm{tgt}}^{(A,B)}(r)] \nabla_{\boldsymbol{\theta}^{(A,B)}} \beta u^{(A,B)}(r|\boldsymbol{\theta}^{(A,B)}) \tag{S8c}$$

where dummy position coordinate $r$ indicates the separation between a pair of particles, $V$ indicates system volume, $N^{(k)}$ indicates particle component number, $\rho^{(k)}$ corresponding component number density, and $g^{(k,k')}(r)$ indicate radial distribution functions. Finally, plugging back each corresponding gradient above into eq. S6 and absorbing all constants in front of each integral as $\alpha^{(k,k')}$, we obtain the parameter update protocol shown as eq. 1 in the main text.

## II. DETERMINING THE RANGES OF OPTIMIZED PAIR INTERACTIONS

The pair separation cut offs for AA, AB, and BB interactions that constrain their respective ranges in the optimizations were initially set to span a finite but large number of coordination shells depending on the openness and complexity of the target lattice. If satisfactory assembly was not achieved, this range was increased. However, if assembly was achieved during the initial optimization, then the cut offs for the interactions were individually reduced to include one less coordination shell in a subsequent optimization. This process was repeated until a minimum number of coordination shells spanned equally by all interaction types for successful target lattice assembly was established. At that point, individual interaction ranges were reduced in subsequent optimizations by a single coordination shell, leaving the other cut offs fixed, until a minimum number of coordination shells was determined for each interaction. As an example, for the triangular honeycomb binary lattice, all interaction ranges were initially set to span five coordination shells, but this number was reduced to two coordination shells after a few successful optimizations. Individual interaction ranges were then independently reduced in subsequent runs. In the end, we found that successful assembly of this lattice could be achieved with cutoffs that included one and two

coordination shells for the AA and BB interactions, respectively. The cross interaction cut off was chosen to span the largest number of coordination shells of individual component self interactions (in this case, two).

## III. GLOBAL TARGET ASSEMBLY FROM SINGLE COMPONENT INTERACTIONS

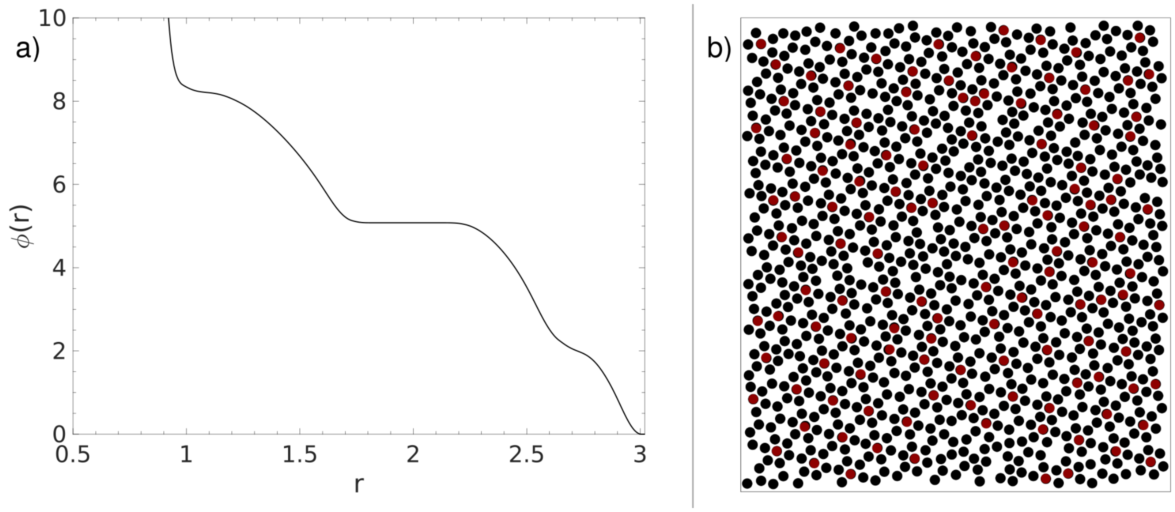


FIG. S1. Single component optimization with global triangular honeycomb as the target structure. The resulting interaction is shown in a) and the corresponding particle self-assembly from the fluid state shown in b). Particles with six neighbors have been colored to aid comparison with the correct local triangular lattice spanned by the A component in the binary structure.

As argued in the main text, stabilizing a global structure featuring two distinct lattice sites is more easily achieved with a binary system whose components independently occupy each such site. Such natural portioning then leads to simpler component interactions than those from a single component system achieving the same equivalent global structure. An example of this argument is shown in figure S1 where we show the interaction obtained from a single component system optimized to stabilize the triangular honeycomb structure from the main text. As seen in a), the potential displays numerous shoulder features that span a total of five target shells. The corresponding particle assembly, with particles displaying six neighbors colored for contrast, is shown in b). Clearly, while the 'honeycomb' matrix is visible throughout the system, the additional 'triangular' ordering from particles occupying

the second site is highly defective. Increasing the optimized interaction range to span as many as nine coordination shells, known to be necessary for other complex single component systems, does not improve ordering and results in assemblies comparable to that shown in figure b). As such, this result provides a substantive example of a single-component system largely failing to stabilize a target that is easily achieved by a binary system using much simpler pair interactions.

## IV. ADDITIONAL OPTIMIZATION RESULTS FOR WCA-LIKE FIXED INTERACTIONS

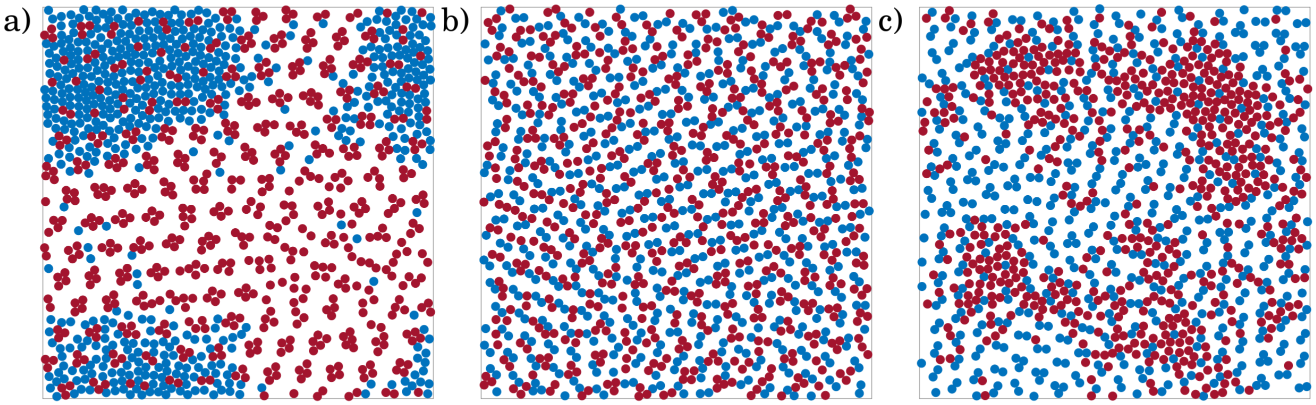


FIG. S2. Assemblies for square truncated hexagonal target (see figure 3 bottom in main text) where a) AA, b) AB , or c) BB interactions have been fixed to display a simple WCA-like repulsion form while the remaining interactions are fully optimized. Target assembly is not achieved in any of these cases.

In figure S2 we show the resulting assemblies when one of the components was fixed to display a WCA-like potential for the STH target. Note that while global assembly fails, local structure can be seen for the non-fixed component such as in a) where BB interactions are optimized and promote assembly of the expected clusters (see Fig. 4 (middle) in the main text) while the A component, whose interaction is fixed, simply phase separates. A similar case applies to c) while b) highlights that coupling is necessary for global assembly despite both A and B having optimized self interactions.

## V. EXAMPLE OF HOW A BINARY SYSTEM CAN ASSEMBLE A TARGET LATTICE WITH SIMPLER OPTIMIZED INTERACTIONS

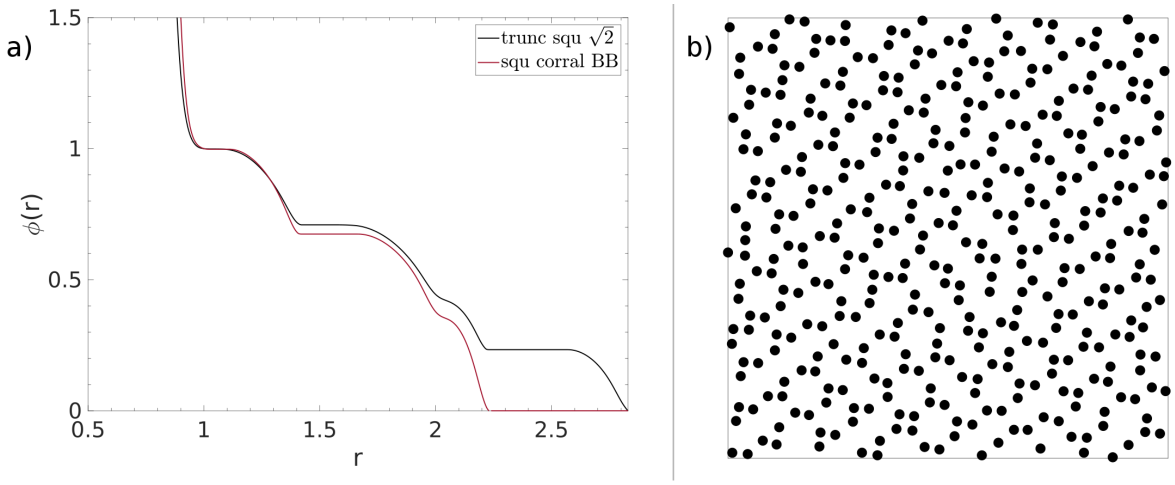


FIG. S3. a)Potentials for the BB square corral interaction (red) and the single component interaction (black) that forms the equivalent local stretched truncated square structure with side ratio $b/a = \sqrt{2}$. Potentials are re-scaled such that $\phi(r)/\phi(1) = 1$. b) Single component particle assembly from the fluid state using the optimized interaction in a).

We provide one example demonstration here for how interactions optimized to assemble a target lattice from a binary system can be simpler than those from a single-component material. We look specifically at the square corral target whose B component forms a stretched truncated square ($b/a = \sqrt{2}$) lattice as its local structure. As shown in figure S3 a), while for the binary square corral system the equivalent truncated square ordering could be achieved with an interaction spanning four coordination shells, the equivalent single component system required five (i.e. a longer ranged interaction). Additionally, the resulting assembly from the single component system using the longer ranged interaction displayed poorer assembly than the coupled, two-component counterpart. We expect similar results for other complex targets, like STH, whose local A component target is a more challenging stretched truncated square $b/a \sim 3.15$, but the optimized AA interaction still only needed to span three coordination shells in the binary system to achieve satisfactory assembly.

## VI. USING SINGLE COMPONENT INTERACTIONS TO BOOST BINARY STABILITY

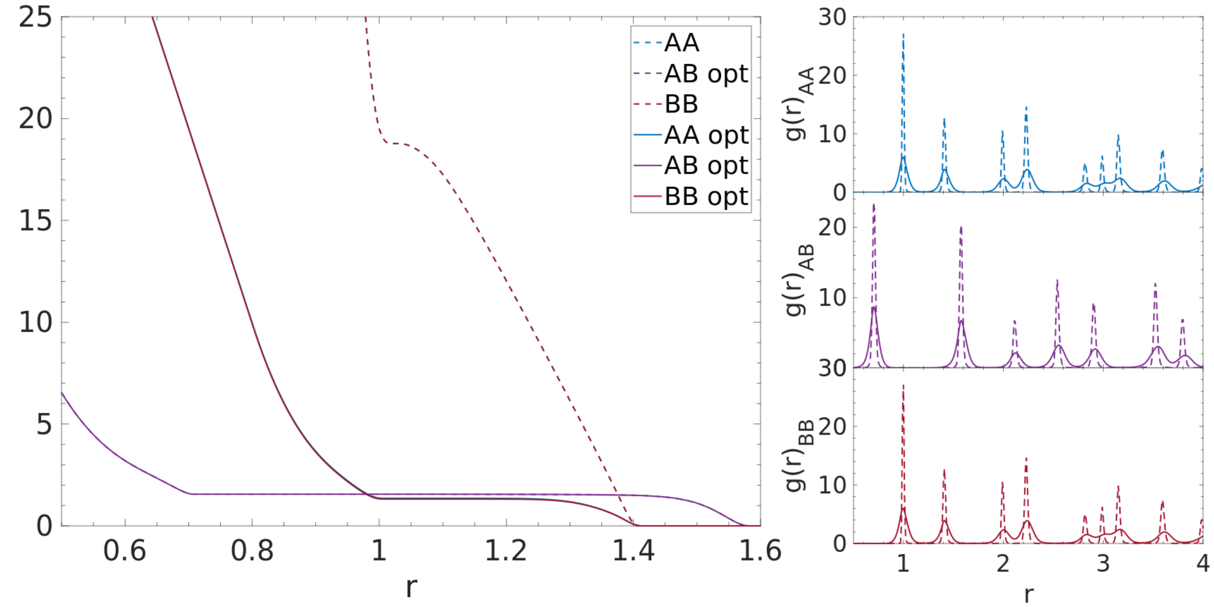


FIG. S4. Potentials for the fully optimized square binary system (solid lines) and an equivalent system but with AA and BB interactions replaced for the single component square lattice forming potential (dashed). Note that potentials AA and BB are identical by symmetry, while the AB opt interactions are kept the same in both systems. Y axis shown in reduced units. The resulting cross and self radial distribution functions for all interactions are compared on the right.

As elaborated in the main text, it is possible to use a pair potential designed to stabilize a lattice in a single component system and replace it for a component interaction that forms the equivalent local lattice in the full binary system. We carried this out for the square binary, where the AA and BB interactions where replaced by the equivalent single component, square lattice forming interaction while keeping the optimized AB interaction for both systems. Equilibrium binary system assembly was then carried out from the fluid state. As seen in figure S4, replacement of the AA and BB interactions with a square lattice forming potential led to dramatic increase in overall binary crystal configurational stability (much sharper peaks in the radial distribution functions). These results therefore directly demonstrate that self interactions can in principle assume the ideal single component forming potential, but need not reach these ideal limits to achieve the full binary system assembly.

Instead, as explained in the main text, the local interactions only need to encode necessary local lengthscales while the coupled interactions drive the larger system into the proper global configuration.

## REFERENCES

[S1] B. A. Lindquist, R. B. Jadrich, and T. M. Truskett, The Journal of Chemical Physics **145**, 111101 (2016), http://dx.doi.org/10.1063/1.4962754.
